# Supplementary material for: BATS: Best Action Trajectory Stitching
Source: arXiv:2204.12026 source file (2022-04-26)
Supplement: Supplementary file 2 [file method_appendix.tex]

\section{The BATS Algorithm}
\label{s:subroutines}

Below we state the steps of the BATS algorithm. Algorithm~\ref{algo:bats} shows the main loop, while Algorithm~\ref{algo:subroutines} shows the subroutines.

\begin{algorithm}
\caption{The BATS Algorithm}
\label{algo:bats}
\begin{algorithmic}
\Procedure{BATS}{Offline Dataset $D = \bigcup_{j \in [M]}\{(s_{ji}, a_{ji}, s'_{ji}, r_{ji})\}_{i=1}^{t_j}$, Max Stitching Length $K$, Number of Iteration $n$, Number of Samples per Iteration $m$, Neighborhood Radius $\epsilon$, Planning Tolerance $\delta$, Discount Factor $\gamma$, Penalty Coefficent $c$, and Distance Metric $d$} \\
% \State $M_0 = \langle \bigcup_{i, t}(\{s_{it}\}\cup\{s'_{it}\}), \left \{ \Actionspace_{s_{it}} =
% \{a_i\} \right\},\gamma, T(s_{it}, a_{it}) = s'_{it}, R(s_{it}, a_{it}) = r_{it}, U(\{s_{i0}\}_{i=1}^N)\rangle$
\State $M_0 = \langle \Statespace_0, \{\Actionspace^s_0\}_{s \in \Statespace_0}, \gamma, T_0, r_0, \rho_0\rangle$
\State \textrm{Learn dynamics estimate, $\tilde{T}$, and reward estimate, $\tilde{r}$ from $D$}
\For{$i = 0, 1, \ldots, (n - 1)$}
    \State $\hat{V}_i^*(\cdot), \pi_i(\cdot) \gets \textrm{valueIteration}(M_i)$
    \State neighbors $\gets \getNeighbors(\Statespace, \pi, M_i, \epsilon)$
    \State $M_{i + 1} \gets M_i$
    \For{$j=1, 2, \ldots, m$}
        \State $s \sim \mu_{M_i}(s \mid \pi_i)$
        \State $E \gets \getPotentialEdges(s, M_i, \text{neighbors}, j)$
        \ForAll{$(s, s') \in E$}
            \State actions = $\testEdge((s, s'), K, \delta)$
            \State $s'' = s$
            \ForAll{$a \in$ actions}
                \State $\Actionspace_{i + 1}^{s''} \geq \{a\} \cup \Actionspace_{i + 1}^{s''}$
                \If{$a$ is last action in actions}
                    \State $T_{i + 1}(s'', a) \gets \tilde{T}(s'', a)$
                    \State $r_{i + 1}(s'', a) \gets \tilde{r}(s'', a) - c d \left( \tilde{T}(s'', a), T(s'', a) \right)$
                    \State $s'' \gets \tilde{T}(s'', a)$
                    \State $\Statespace_{i + 1} \gets \{s''\} \cup \Statespace_{i + 1}$
                \Else
                    \State $T_{i + 1}(s'', a) \gets s'$
                    \State $r_{i + 1}(s'', a) \gets \tilde{r}(s'', a) - c d \left( \tilde{T}(s'', a), s' \right)$
                \EndIf
            \EndFor
        \EndFor
    \EndFor
\EndFor
\State $V(\cdot), \pi(\cdot) \gets \textrm{valueIteration}(M_n)$
\Return $M_n$
\EndProcedure

\end{algorithmic}

\end{algorithm}

\begin{algorithm}
\caption{Subroutines for BATS}
\label{algo:subroutines}
\begin{algorithmic}
\Function{$\getPotentialEdges$}{$s, t, \hat{M}, \text{neighbors}, j$}
\If{k == 0}
    \Return []
\EndIf
\State edges = []
\State vertexNeighbors $\gets$ $\text{neighbors}[t]$
\State MDPNeighbors $\gets \hat{M}[s, \hat{\Actionspace}_s]$
\ForAll{$n \in$ vertexNeighbors}
    \State edges += $\getFutureEdges$($s$, $n$, $\hat{M}$, $j$)
\EndFor
\ForAll{$n \in$ MDPNeighbors}
    \State successorNeighbors $\gets \text{neighbors}[t]$
    \ForAll{$n' \in$ successorNeighbors}
        \State neighbors += [($s$, $n'$)]
    \EndFor
    \State neighbors += $\getPotentialEdges(s, n, \hat{M}, \text{neighbors}, j - 1)$
\EndFor

\Return edges
\EndFunction
\Function{$\getFutureEdges$}{$s, n, \hat{M}, j$}
    \State MDPNeighbors $\gets \hat{M}[s, \hat{A}_s]$
    \State edges $\gets$ []
    \ForAll{$n' \in$ MDPNeighbors}
        \State edges += $[(s, n')]$
        \State edges += $\getFutureEdges(s, n', \hat{M}, j-1)$
    \EndFor

\Return edges
\EndFunction
\Function{$\testEdge$}{e, k, $\epsilon$}
    \State minDistance $\gets \infty$
    \State bestActions $\gets []$
    \For{i = 1:j}
        \State distance, actions $\gets \CEM(e, k)$
        \If{distance < minDistance}
            \State minDistance $\gets$ distance
            \State bestActions $\gets$ actions
        \EndIf
    \EndFor
    \If{minDistance < $\epsilon$}
        \Return []
    \EndIf
    
    \Return bestActions
\EndFunction
\end{algorithmic}
\end{algorithm}

\newpage
